# Supplementary material for: MMCR: Advancing Visual Language Model in Multimodal Multi-Turn Contextual Reasoning
Source: arXiv:2503.18533 source file (2025-03-24)
Supplement: Supplementary file 1 [file x_supp.tex]

\clearpage
\setcounter{page}{1}
\setcounter{figure}{0}
\setcounter{section}{0}
\setcounter{table}{0}

\maketitlesupplementary

\begin{figure*}[ht]
    \centering
    \includegraphics[scale=0.21]{ICCV2025-Author-Kit-Feb/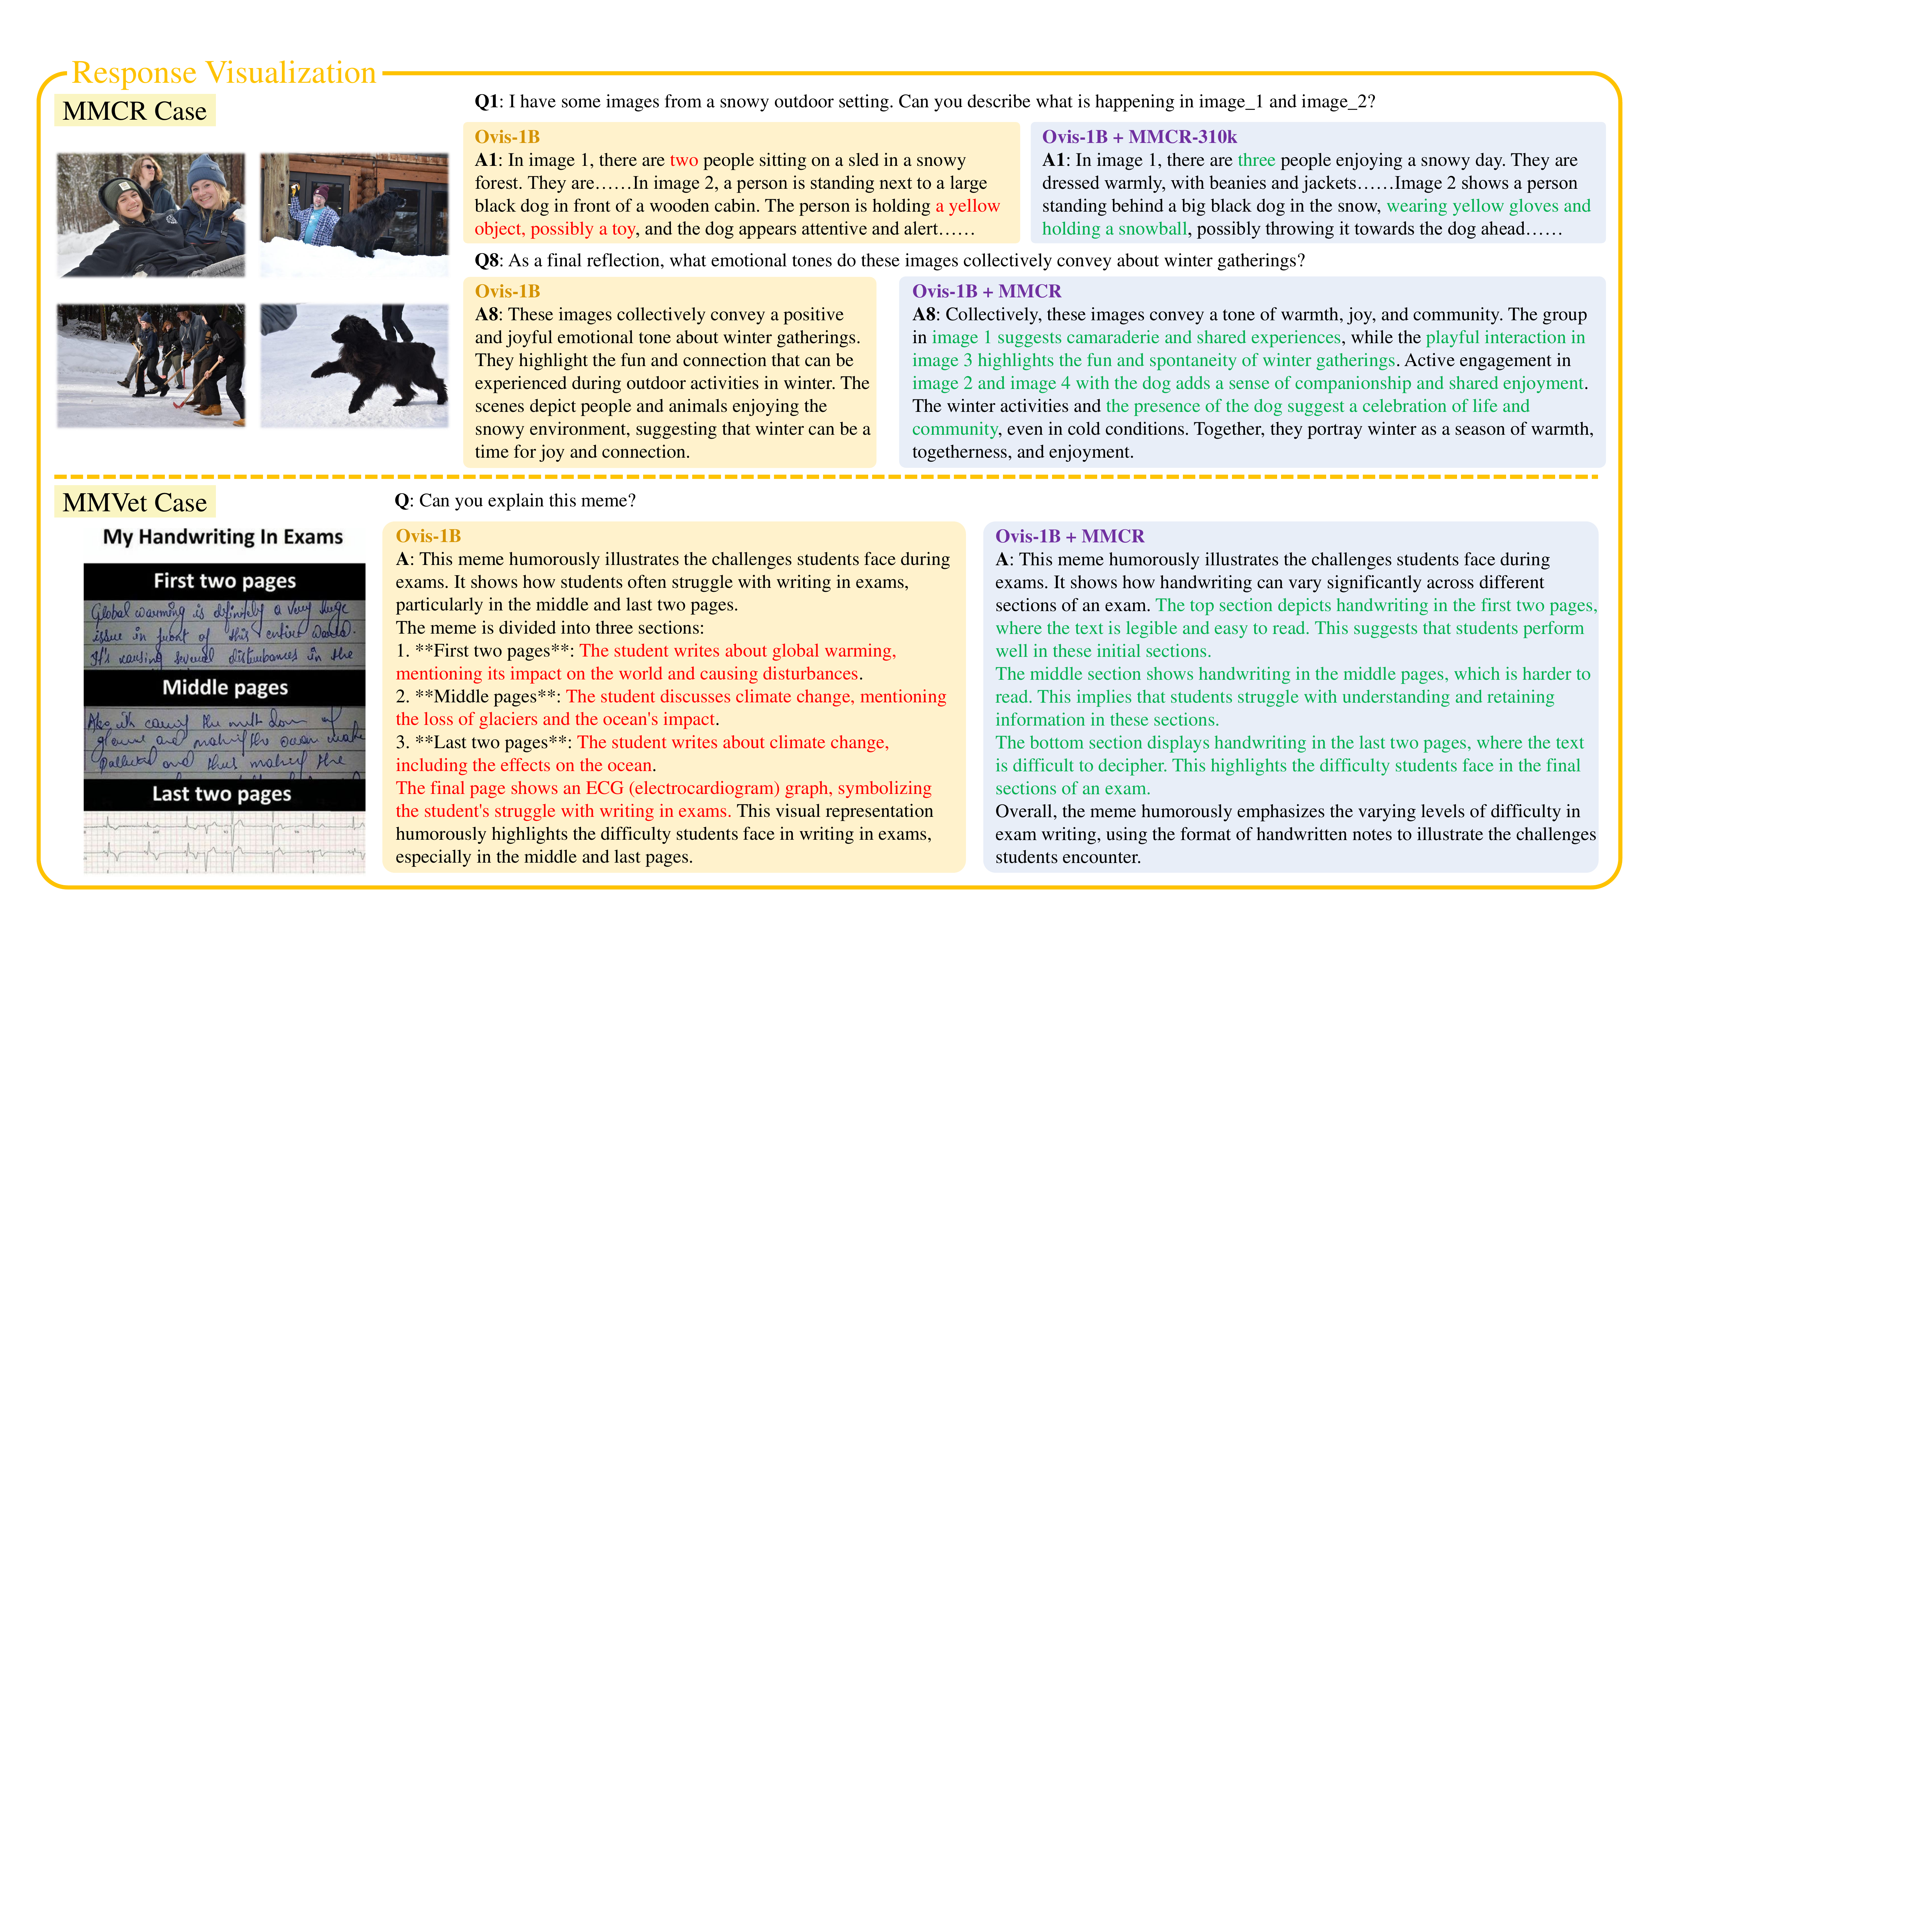}
    \caption{Visualization of Response Comparison. We present a comparison between the baseline Ovis-1B and the model fine-tuned with MMCR data. Errors and hallucinations are marked in \textcolor{red}{red}, while detailed and accurate descriptions are marked in {\color[HTML]{0ADF0B} green}.}
    \label{fig:visual}
\end{figure*}

\section{Implementation Details}
We use Ovis as the baseline model for all experiments. Ovis encompasses three configurations: the LLM module, the ViT backbone, and the visual vocabulary size. We incorporate popular open-source LLM (Qwen2.5-Instruct~\cite{qwen2025qwen25technicalreport} and ViT (aimv2~\cite{fini2024multimodalautoregressivepretraininglarge}) into Ovis. The size of the visual vocabulary is set to 65536. 
We strictly adhere to the original Ovis settings to ensure fairness. The batch size is 1024, with 1 epoch. The experiments use a cosine annealing learning rate of 2e-6 and a weight decay of 0. All experiments are conducted using the PyTorch framework on 8 H100 80G GPUs.

% \section{Related Benchmarks}

\section{Response Visualization}
We visually demonstrate the optimizations brought by MMCR through model responses. Fig.~\ref{fig:visual} shows a comparison between the baseline and MMCR-enhanced model responses on two evaluation datasets—MMCR-Bench and MMVet. It is evident that after incorporating MMCR data, the model’s responses become more accurate and clear, effectively mitigating issues of hallucination and vague understanding. The improved responses reveal a deeper comprehension of the underlying meanings in the images, rather than merely interpreting their symbolic shapes.

\section{Generate prompt}
We have meticulously designed a prompt for GPT-4o to generate multi-image, multi-turn dialogues with strong contextual relevance, thereby more efficiently utilizing the provided images and text. The exact prompt is shown in Fig.~\ref{fig:generate_prompt}. First, we define the task: the agent must simulate a real-world scenario where a human provides images, background information, and their own requests in an interaction with an intelligent assistant. The key requirement is that the overall dialogue maintains clear contextual continuity, with subsequent questions based on previous requests or questions and their corresponding answers, which aligns with the original intention behind designing MMCR. Second, to ensure that the generated data can be effectively used for the instruction fine-tuning phase of VLMs, we emphasize that only the human should introduce images, and images with significantly disparate content should be distributed across multiple dialogue turns to avoid abrupt transitions. Since the accuracy of the assistant's responses—ensuring that they are consistent with the provided data and free from hallucinations or creative interpretations—is crucial for the dataset's quality, we require that the generated dialogues adhere strictly to the provided data without introducing fictional content.
Next, we stress the importance of adhering to a standardized data format and avoiding any content that may contain harmful elements. Finally, to ensure the overall quality of the generated data, we instruct GPT-4o to recheck the generated multimodal, multi-turn dialogues against all the above requirements.
This carefully crafted prompt has proven to be highly effective in guiding the generation process.

\section{Judgment prompt}
In Fig.~\ref{fig:judge_prompt}, we present the prompt used to evaluate the model responses against the reference provided in MMCR-Bench. This prompt guides GPT-4o to assess the responses from six aspects: Precision, Consistency, Logical, Clarity, Redundancy, and Overall Score. Each dimension is divided into five scoring intervals, with corresponding descriptions defined for each interval to enable accurate judgment of the model's performance. Finally, we aggregate the scores from all 600 evaluation samples in MMCR-Bench by summing them, dividing by the total number of samples, and then multiplying by 10 to obtain the final score for the model's responses.

\section{Data Example}
In Fig.~\ref{fig:case_1} and Fig.~\ref{fig:case_2}, we present two multimodal multi-turn dialogue samples from MMCR-310k and MMCR-Bench, respectively, to illustrate the characteristics of our data. Overall, our data features long-duration multi-turn dialogues, involves the understanding and perception of multiple images, maintains rigorous contextual logical relationships, and consistently focuses on discussions around specific images with a clearly defined theme.

Specifically, we use “Image\_n: $\textlangle$image$\textrangle$,” in the dialogue to specify the position for the corresponding image token, where n denotes the specific image number. In the example shown in Fig.~\ref{fig:case_1}, the human’s Question 1 initially involves two images. After prompting the intelligent assistant for descriptions, the conversation expands into a discussion about the lifestyles represented by each image. Subsequently, in Question 3, the third image is introduced, leading to a discussion of the relationships between Image 2 and Image 3, as well as between Image 1 and Image 3, and culminating in a comprehensive discussion that summarizes all the images. This setup challenges the VLM’s ability to understand and retain long texts. Similarly, in the example from Fig.~\ref{fig:case_2}, the human’s question involves multiple images and ultimately revolves around the central dialogue theme. These examples not only highlight the challenges of long-text understanding and memory for VLMs but also provide a comprehensive evaluation of the model’s contextual reasoning and multi-image perceptual understanding capabilities.

\begin{figure*}[t]
    \centering
    \includegraphics[scale=0.32]{ICCV2025-Author-Kit-Feb/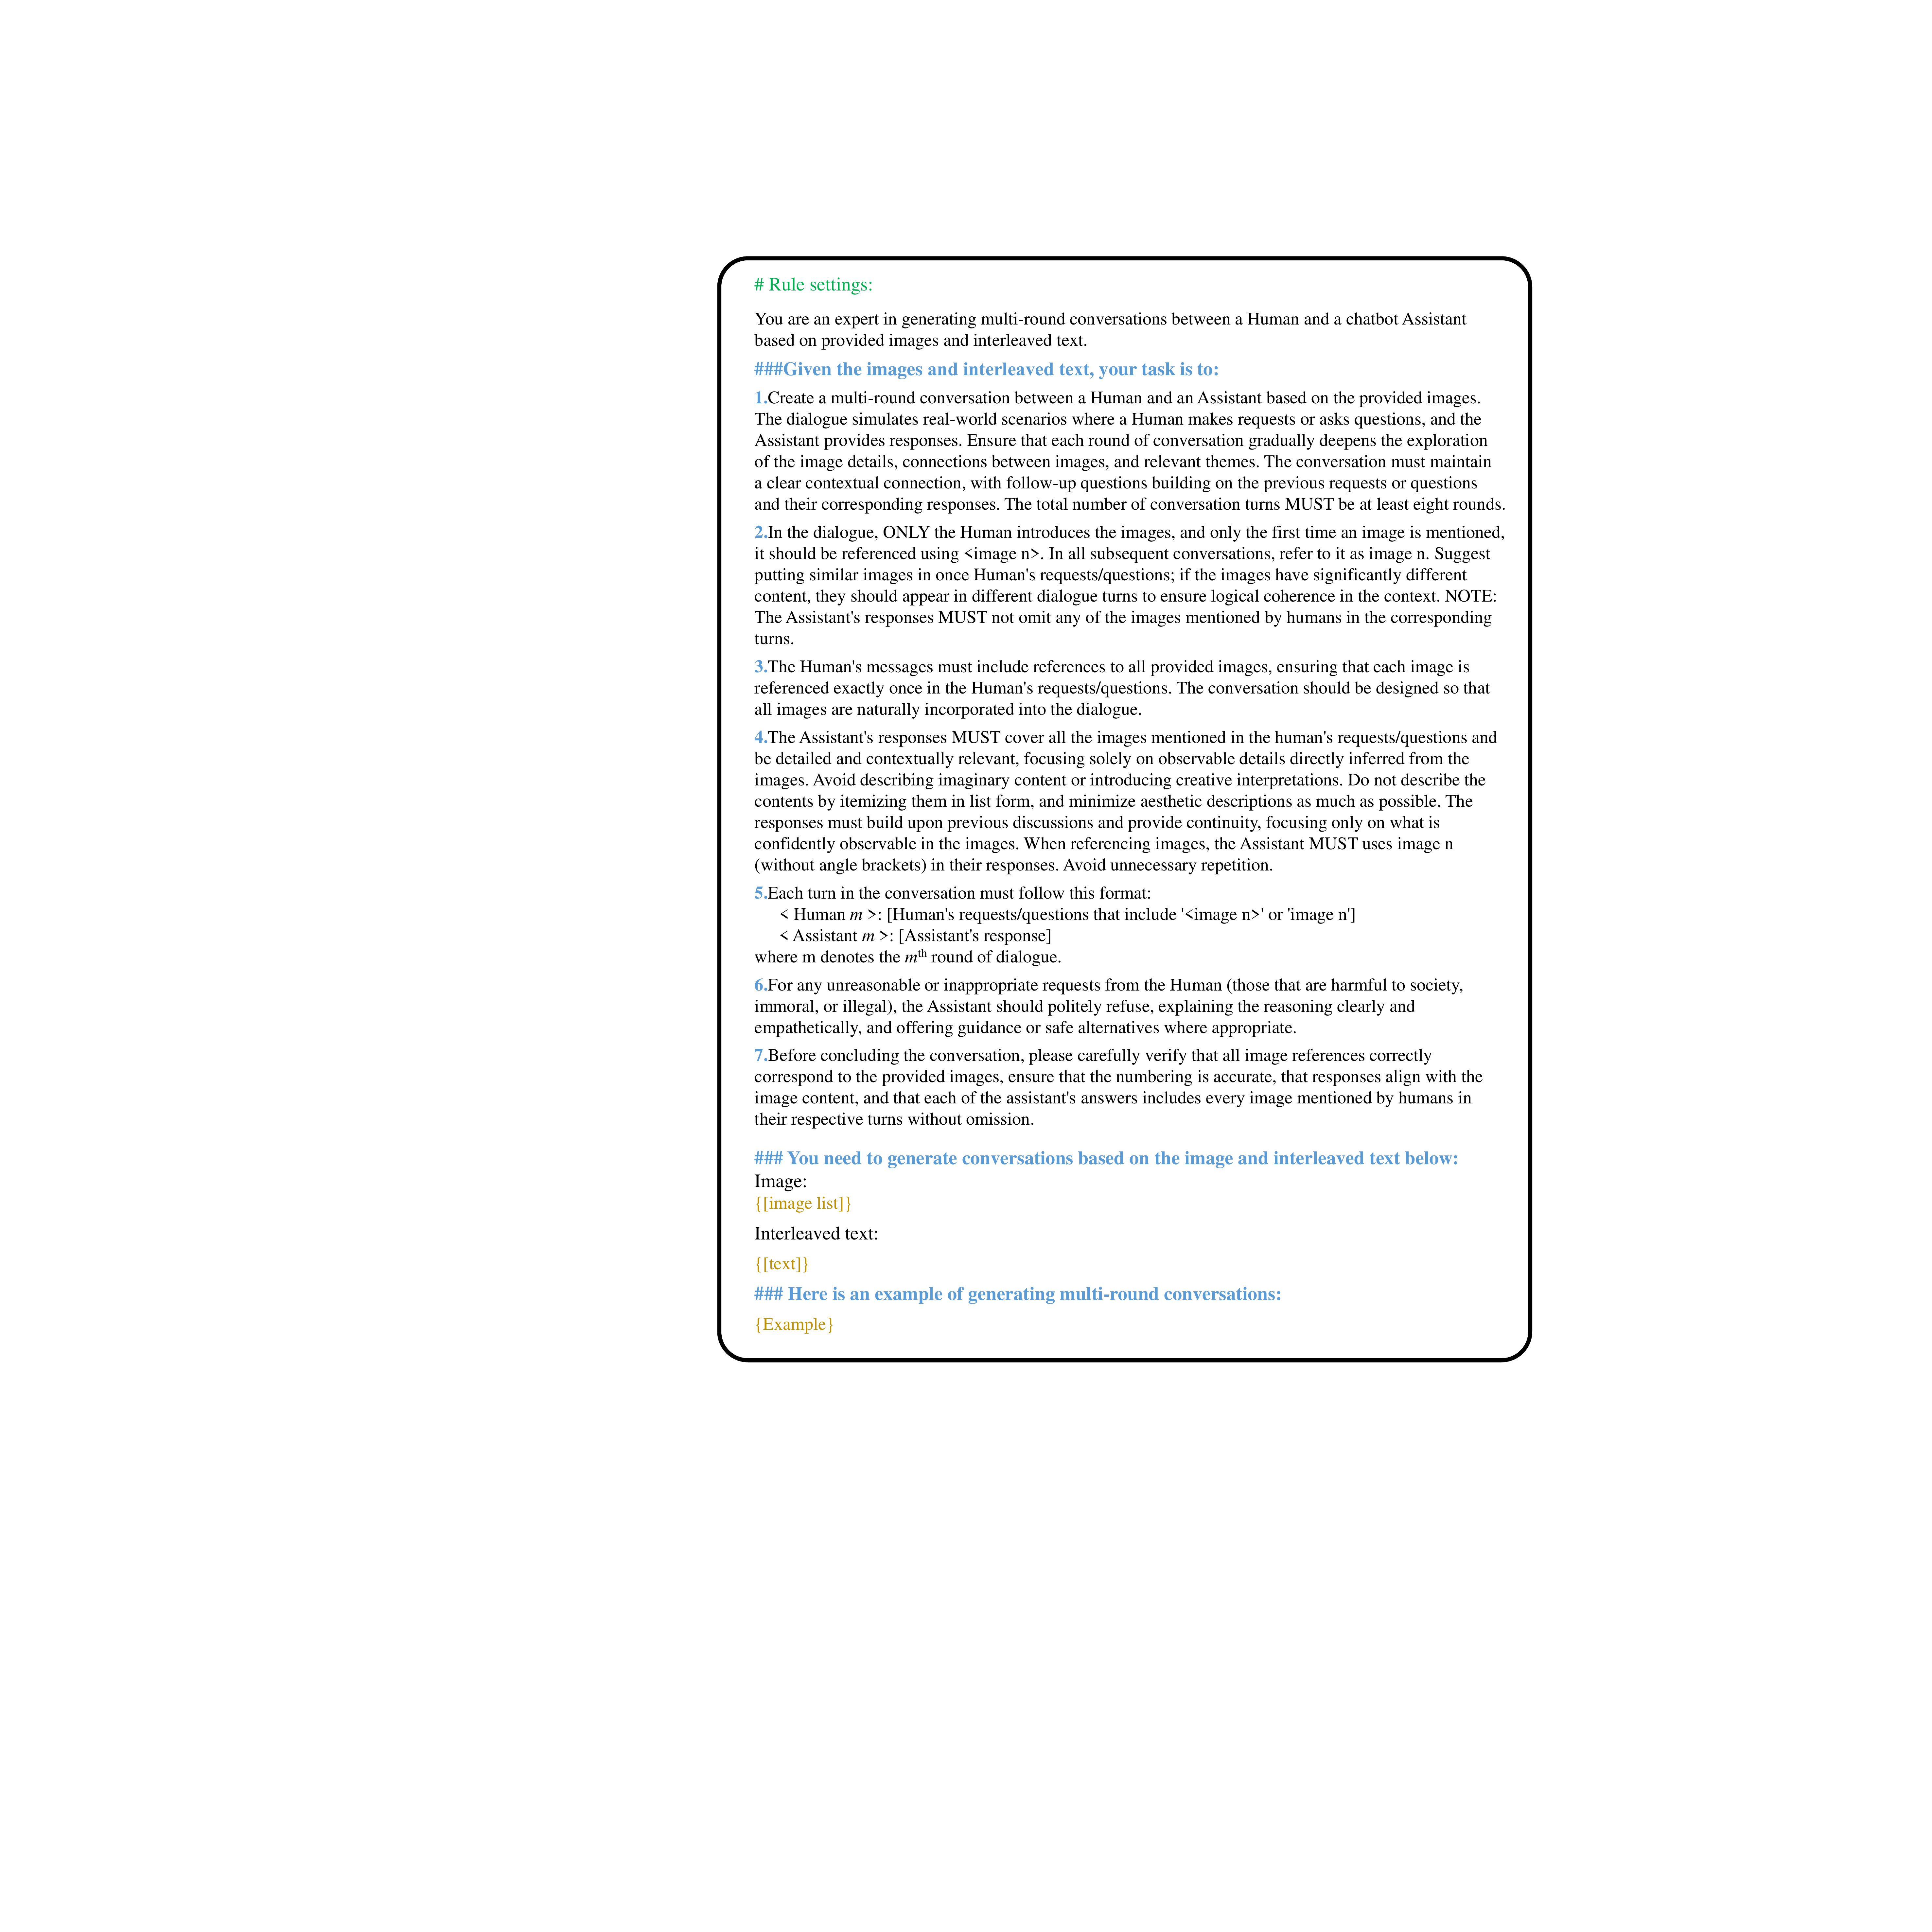}
    \caption{Dialogue generation prompt.}
    \label{fig:generate_prompt}
\end{figure*}

\begin{figure*}[t]
    \centering
    \includegraphics[scale=0.32]{ICCV2025-Author-Kit-Feb/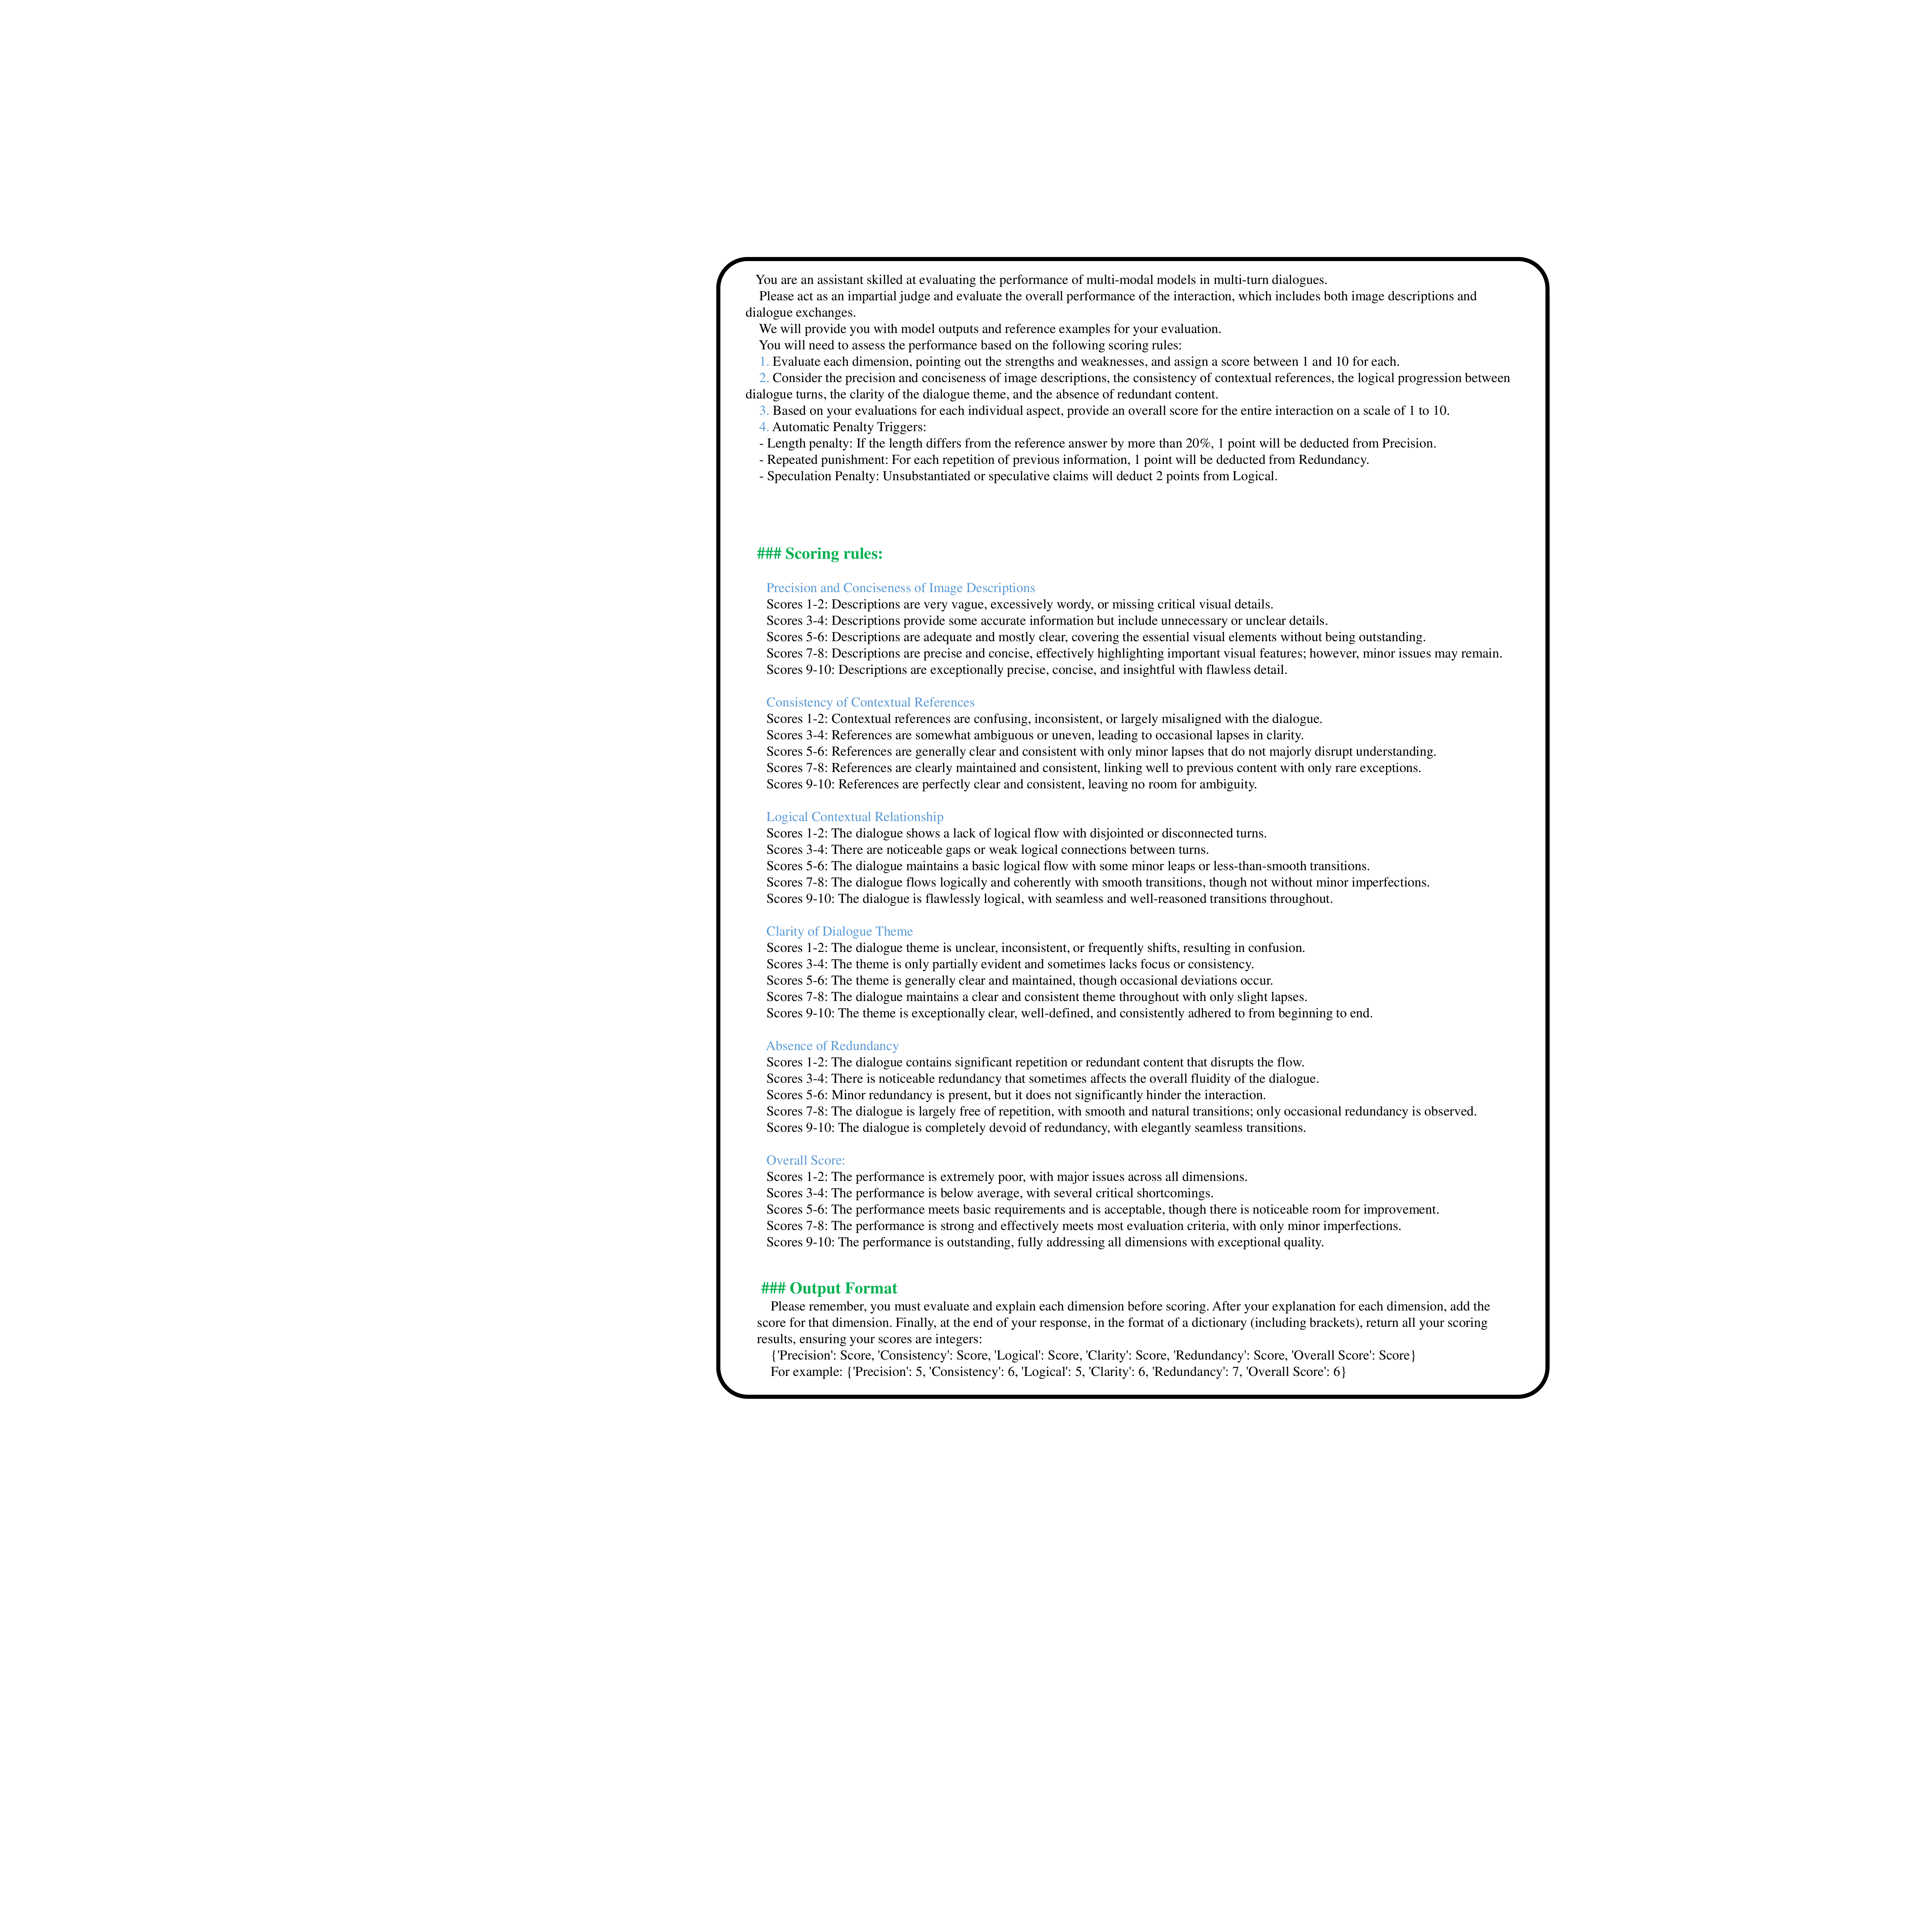}
    \caption{Judgment prompt for GPT-4o.}
    \label{fig:judge_prompt}
\end{figure*}

\begin{figure*}[t]
    \centering
    \includegraphics[scale=0.28]{ICCV2025-Author-Kit-Feb/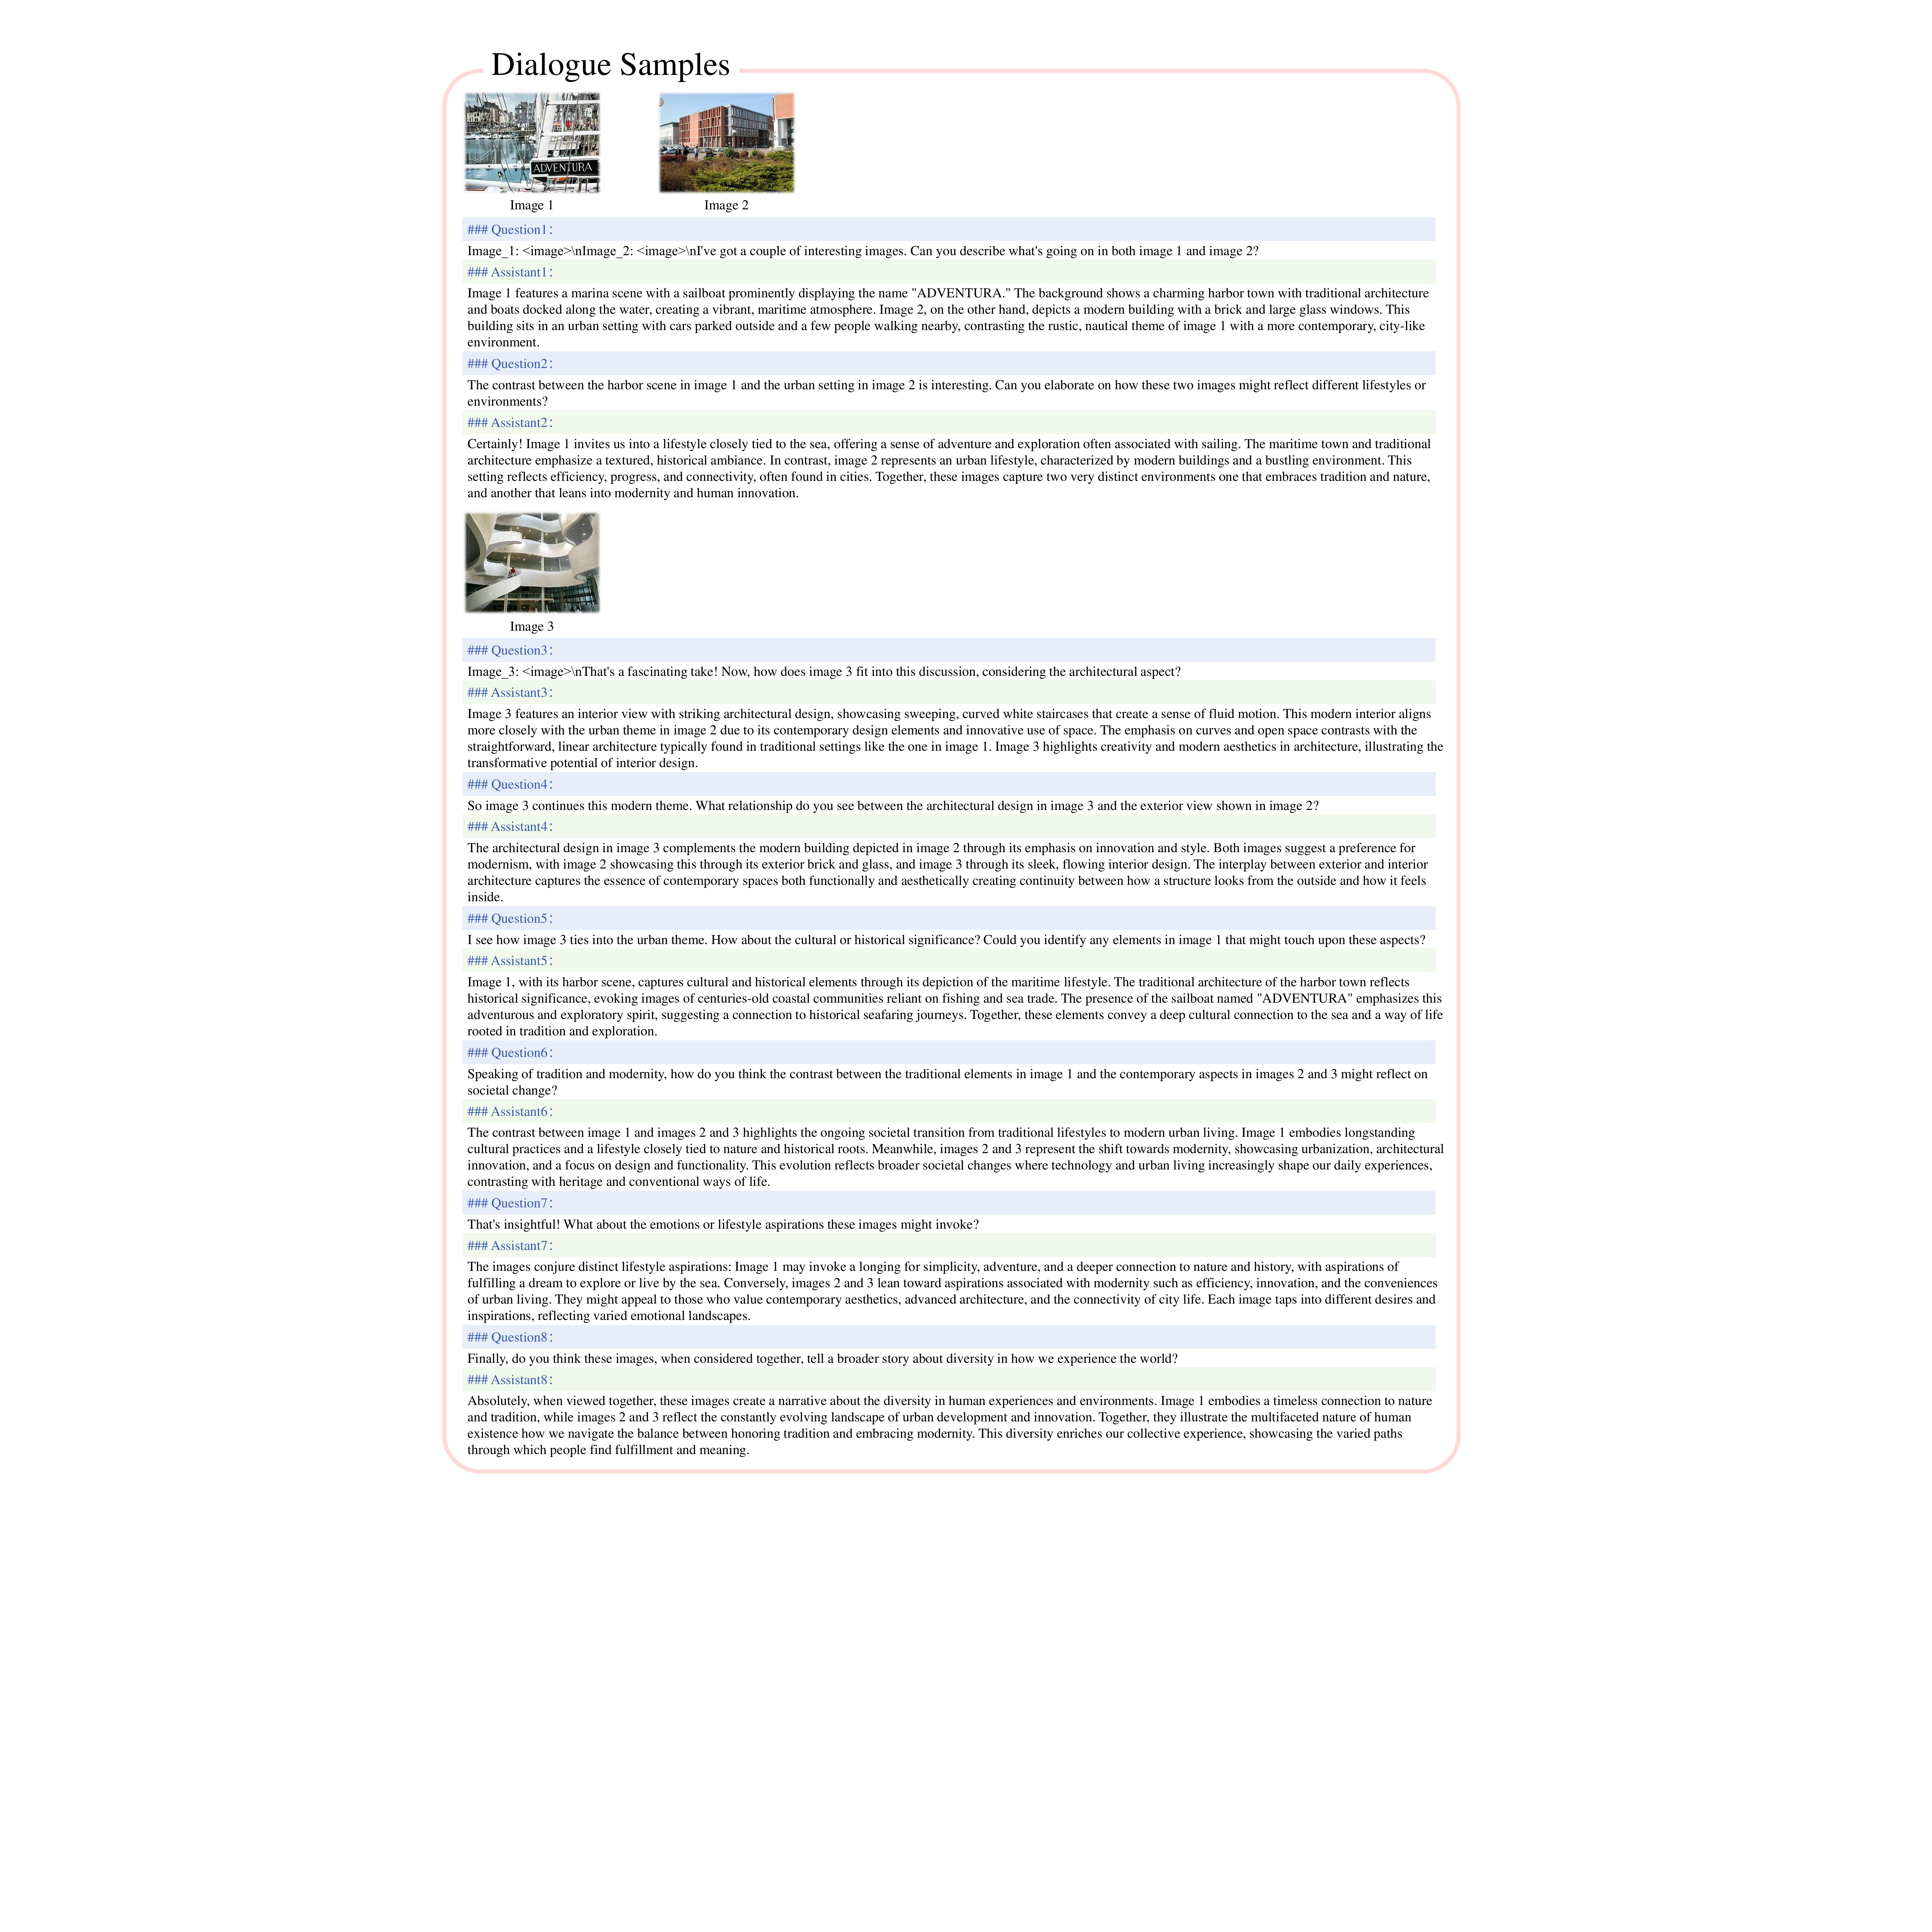}
    \caption{MMCR-310k Example.}
    \label{fig:case_1}
\end{figure*}

\begin{figure*}[t]
    \centering
    \includegraphics[scale=0.28]{ICCV2025-Author-Kit-Feb/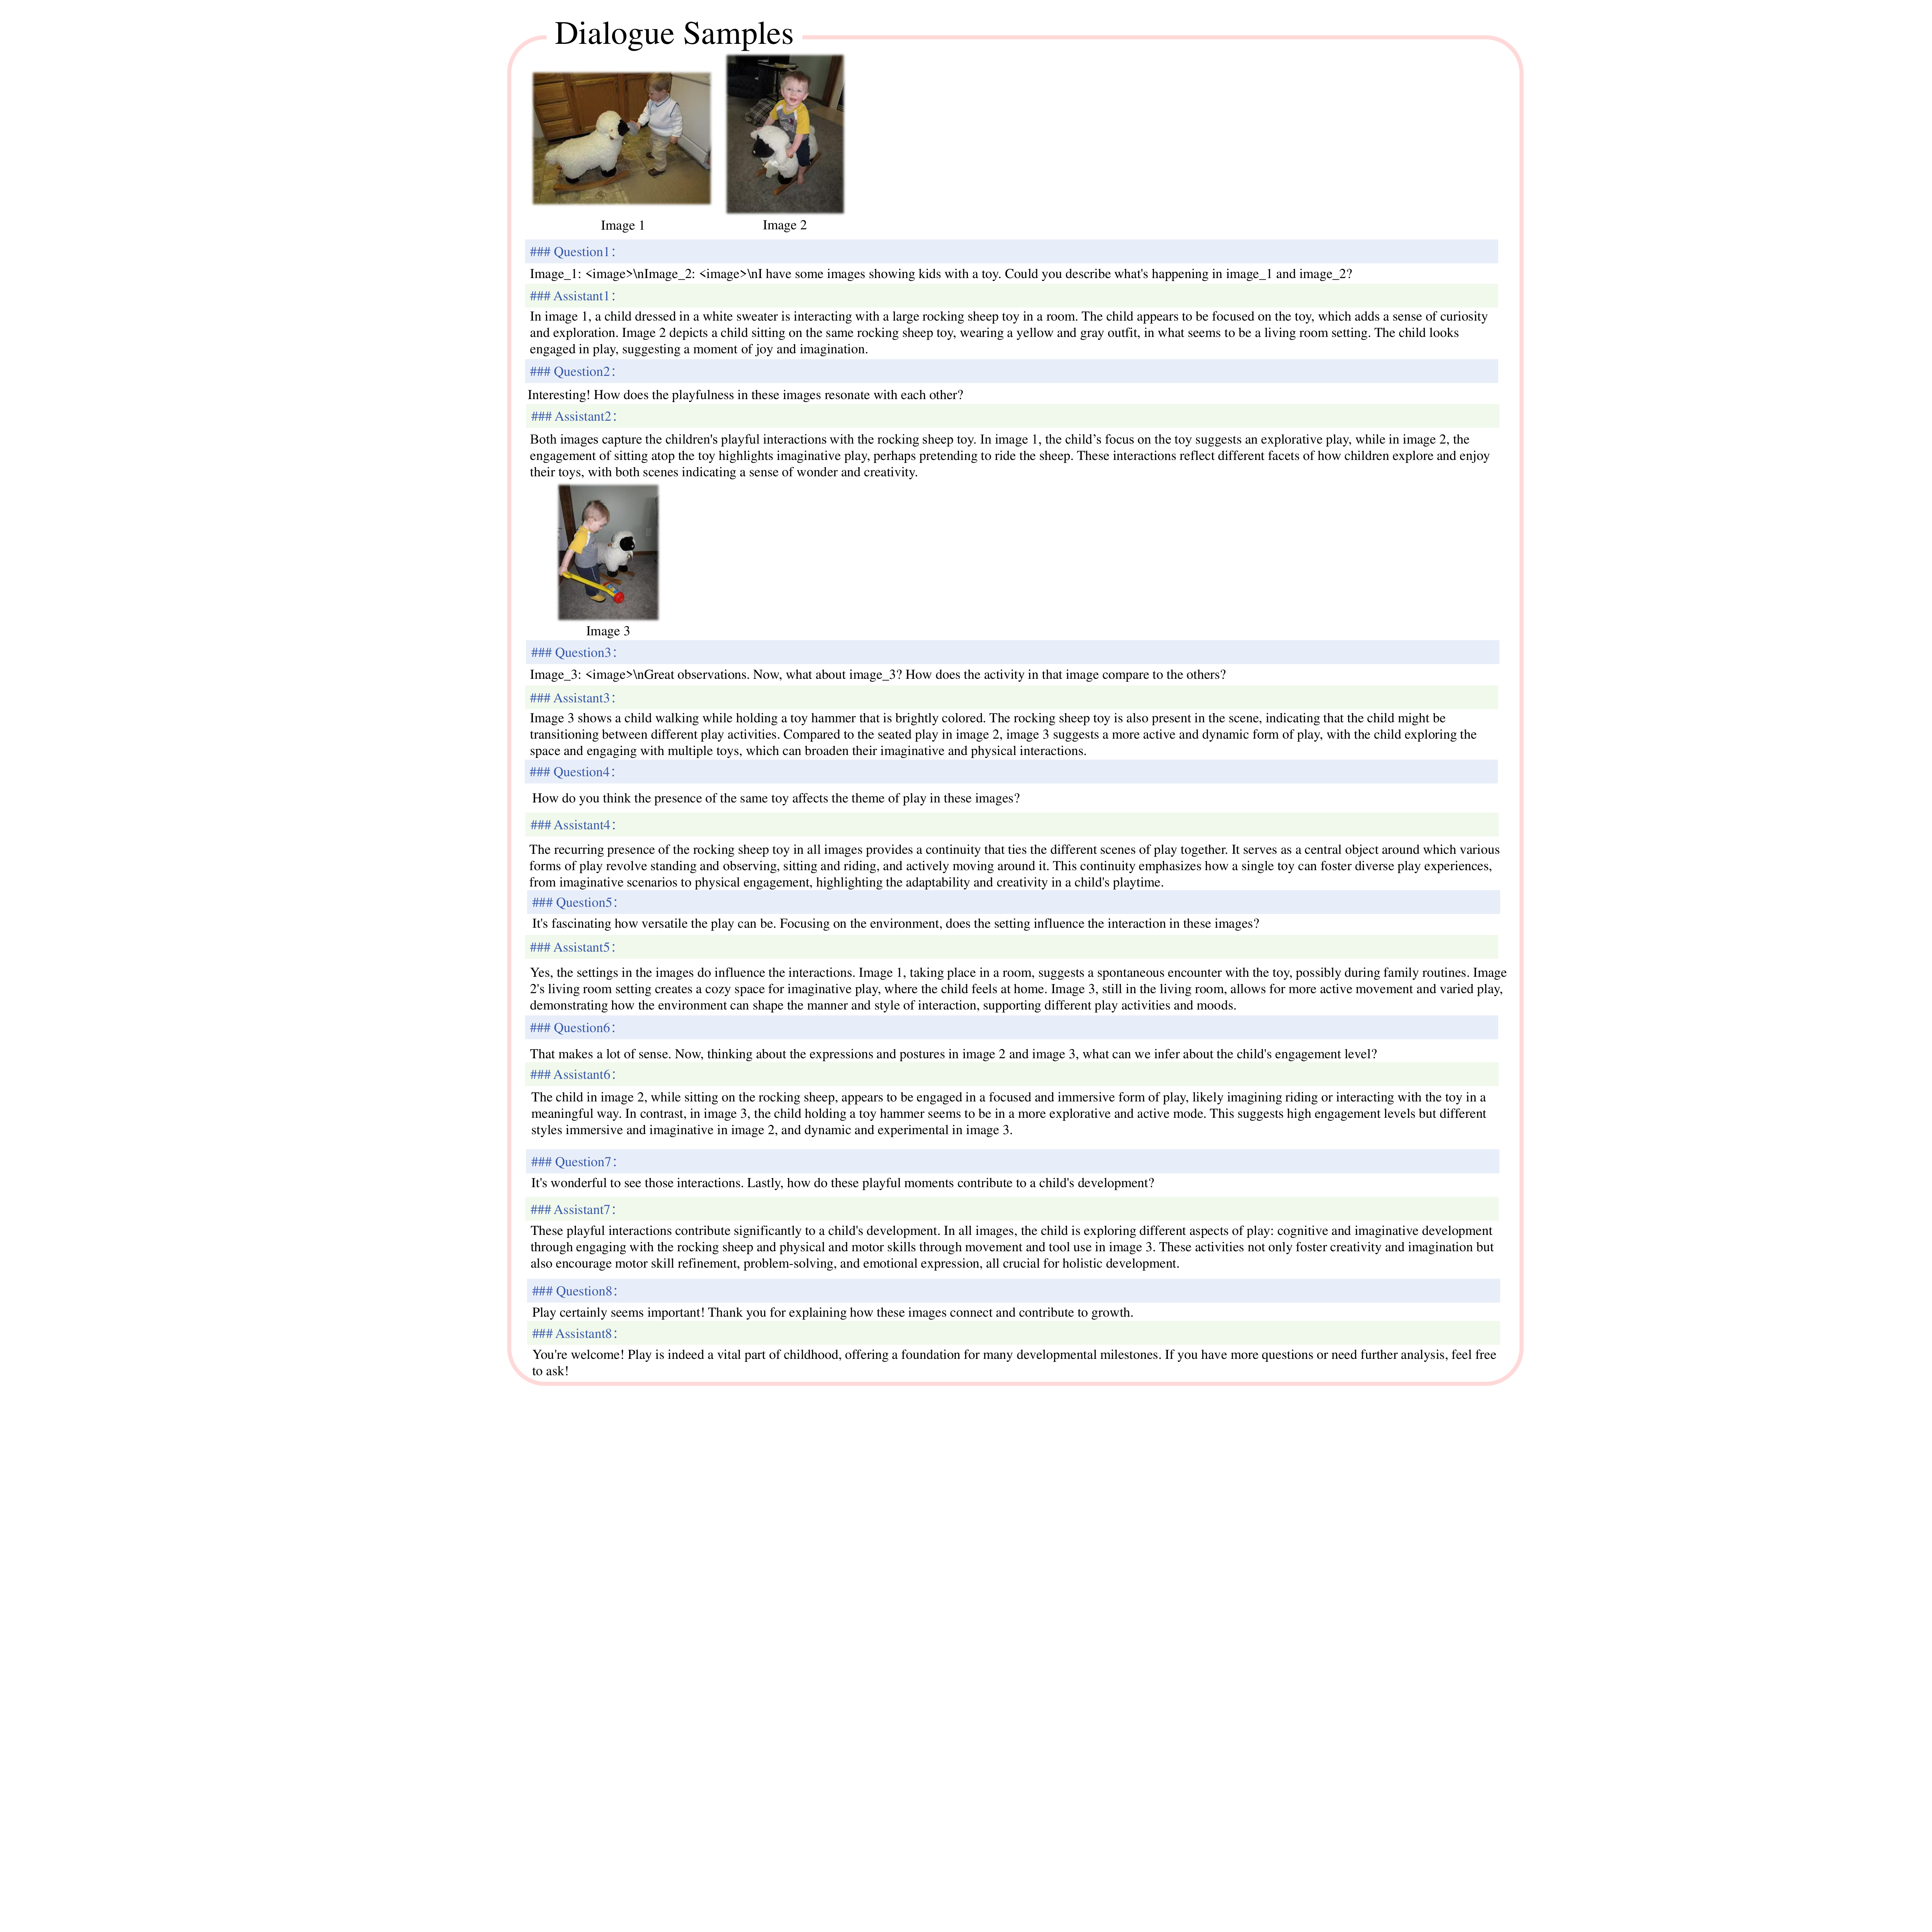}
    \caption{MMCR-Bench Example.}
    \label{fig:case_2}
\end{figure*}
